# Supplementary material for: Scale and Scheme Independence and Position-Momentum Equivalence of Nuclear Short-Range Correlations
Source: arXiv:1907.03658 ancillary file (2021-01-14)
Supplement: Supplementary file 1 [file Supplementary_v2.pdf]

# Supplementary Materials: Scale and Scheme Independence and Position-Momentum Equivalence of Nuclear Short-Range Correlations

## SHORT-R, HIGH-K BEHAVIOR FOR DIFFERENT NN INTERACTIONS

The figure below shows how ab-initio many-body calculations using different models of the nucleon-nucleon ($NN$) interaction produce nuclear wave-functions that differ significantly at high-momenta and at short-distances. This is generally referred to as "scale and scheme dependence".

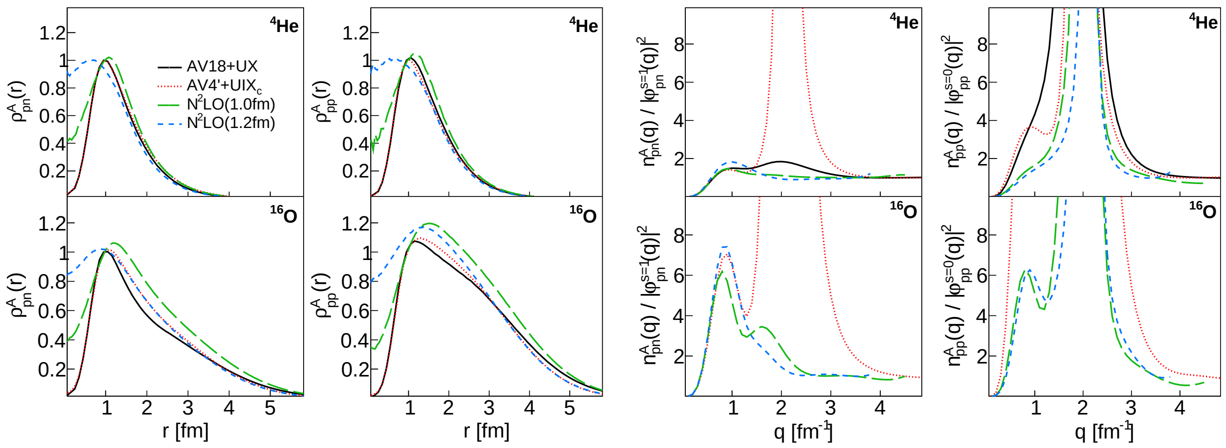


FIG. 1: Two-nucleon coordinate (left two columns) and momentum (right two columns) space distributions calculated using different $NN$+$3N$ potentials for different nuclei. The top and bottom rows show distributions for $^4$He and $^{16}$O respectively.

## DENSITY SCALING FOR nn PAIRS

Figure 2 shows $\rho^{nn}_A(r)$ (left panel) and $n^{nn}_A(q)/|\varphi^{s=0}_{nn}(q)|^2$ (right panel) for all four interactions and different nuclei. The densities in coordinate space were scaled to have the same value at $\sim 1\,\mathrm{fm}$. Similarly, the momentum space densities were scaled to have the same value at $\sim 4\,\mathrm{fm}^{-1}$.

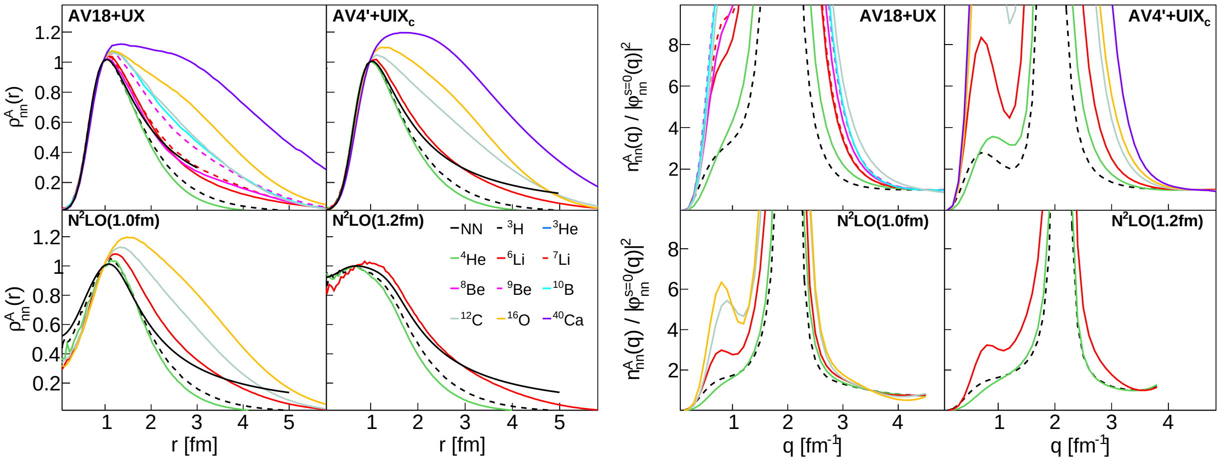


FIG. 2: Two-nucleon coordinate (left) and momentum (right) space distributions for nn pairs calculated using different $NN$+$3N$ potentials for different nuclei.

## EXTRACTED CONTACT VALUES

| | | $C_{pn}^{s=1}$ | | $C_{pp}^{s=0}$ | | $C_{pn}^{s=0}$ | |
|---|---|---|---|---|---|---|---|
| | | r | k | r | k | r | k |
| $D$ | AV18 | 4.898 ± 0.080 | 4.764 ± 0.007 | | | | |
| | AV4' | 1.186 ± 0.034 | 1.165 ± 0.037 | | | | |
| | N$^2$LO(1.0) | 4.664 ± 0.009 | 4.691 ± 0.030 | | | | |
| | N$^2$LO(1.2) | 4.141 ± 0.010 | 4.244 ± 0.032 | | | | |
| $^3H$ | AV18 | 6.246 ± 0.856 | 6.441 ± 0.645 | 0.549 ± 0.055 | 0.590 ± 0.060 | 0.295 ± 0.119 | 0.311 ± 0.033 |
| | AV4' | 1.533 ± 0.154 | 1.515 ± 0.152 | 0.544 ± 0.055 | 0.532 ± 0.054 | 0.270 ± 0.027 | 0.281 ± 0.029 |
| | N$^2$LO(1.0) | 6.237 ± 0.718 | 6.885 ± 0.789 | 0.282 ± 0.032 | 0.521 ± 0.060 | 0.140 ± 0.015 | 0.255 ± 0.063 |
| | N$^2$LO(1.2) | 5.980 ± 0.695 | 6.111 ± 1.011 | 0.277 ± 0.033 | 0.687 ± 0.119 | 0.139 ± 0.017 | 0.337 ± 0.061 |
| $^3He$ | AV18 | 6.851 ± 0.822 | 6.249 ± 0.625 | 0.536 ± 0.054 | 0.570 ± 0.058 | 0.161 ± 0.092 | 0.325 ± 0.034 |
| | AV4' | 1.527 ± 0.153 | 1.466 ± 0.147 | 0.515 ± 0.052 | 0.515 ± 0.052 | 0.265 ± 0.027 | 0.264 ± 0.028 |
| | N$^2$LO(1.0) | 6.113 ± 0.719 | 6.703 ± 0.702 | 0.259 ± 0.032 | 0.454 ± 0.069 | 0.135 ± 0.016 | 0.264 ± 0.047 |
| | N$^2$LO(1.2) | 5.705 ± 0.870 | 5.717 ± 0.730 | 0.239 ± 0.041 | 0.547 ± 0.079 | 0.127 ± 0.022 | 0.307 ± 0.057 |
| $^4He$ | AV18 | 11.605 ± 1.161 | 12.274 ± 1.232 | 0.567 ± 0.057 | 0.655 ± 0.071 | 0.567 ± 0.057 | 0.687 ± 0.075 |
| | AV4' | 2.685 ± 0.272 | 2.995 ± 0.300 | 0.564 ± 0.057 | 0.542 ± 0.055 | 0.578 ± 0.059 | 0.564 ± 0.057 |
| | N$^2$LO(1.0) | 10.508 ± 1.308 | 12.372 ± 1.372 | 0.243 ± 0.040 | 0.655 ± 0.093 | 0.253 ± 0.043 | 0.703 ± 0.096 |
| | N$^2$LO(1.2) | 11.111 ± 2.595 | 10.446 ± 2.223 | 0.263 ± 0.059 | 0.851 ± 0.102 | 0.281 ± 0.062 | 0.934 ± 0.133 |
| $^6Li$ | AV18 | 10.140 ± 1.015 | 10.492 ± 1.056 | 0.415 ± 0.042 | 0.485 ± 0.058 | 0.415 ± 0.042 | 0.529 ± 0.071 |
| | AV4' | 2.248 ± 0.225 | 2.205 ± 0.222 | 0.380 ± 0.038 | 0.380 ± 0.038 | 0.387 ± 0.039 | 0.369 ± 0.039 |
| | N$^2$LO(1.0) | 8.434 ± 1.026 | 9.444 ± 1.141 | 0.173 ± 0.020 | 0.501 ± 0.074 | 0.180 ± 0.021 | 0.540 ± 0.086 |
| | N$^2$LO(1.2) | 9.011 ± 1.478 | 8.650 ± 1.545 | 0.185 ± 0.031 | 0.668 ± 0.104 | 0.197 ± 0.034 | 0.749 ± 0.168 |
| $^{12}C$ | AV18 | 13.135 ± 1.324 | 15.876 ± 1.770 | 0.716 ± 0.075 | 1.140 ± 0.210 | 0.716 ± 0.075 | 1.244 ± 0.319 |
| | AV4' | 2.458 ± 0.249 | 2.676 ± 0.272 | 0.547 ± 0.055 | 0.653 ± 0.067 | 0.559 ± 0.056 | 0.558 ± 0.069 |
| | N$^2$LO(1.0) | 10.434 ± 1.044 | 10.643 ± 1.094 | 0.308 ± 0.033 | 0.870 ± 0.095 | 0.318 ± 0.034 | 0.988 ± 0.161 |
| $^{16}O$ | AV18 | 11.372 ± 1.158 | | 0.676 ± 0.072 | | 0.676 ± 0.072 | |
| | AV4' | 2.910 ± 0.293 | 2.911 ± 0.307 | 0.658 ± 0.066 | 0.784 ± 0.084 | 0.675 ± 0.068 | 0.702 ± 0.086 |
| | N$^2$LO(1.0) | 9.103 ± 1.020 | 10.338 ± 1.310 | 0.270 ± 0.034 | 0.781 ± 0.173 | 0.275 ± 0.033 | 0.928 ± 0.365 |
| $^{40}Ca$ | AV18 | 11.570 ± 1.196 | | 0.723 ± 0.081 | | 0.723 ± 0.081 | |
| | AV4' | 3.284 ± 0.339 | 4.476 ± 0.460 | 0.834 ± 0.084 | 1.329 ± 0.144 | 0.854 ± 0.086 | 1.357 ± 0.164 |

TABLE I: The extracted contact values have been divided by A/2 and multiplied by 100 to give the percent of nucleons above $k_F$. For symmetric nuclei, $C_{nn}^{s=0} = C_{pp}^{s=0}$. In the case of $^3He$, $C_{nn}^{s=0} = 0$, as there is only one neutron in this nucleus. In the case of $^3H$, $C_{pp}^{s=0} = 0$, as there is only one proton in this nucleus, and the values shown under $C_{pp}^{s=0}$ correspond to $C_{nn}^{s=0}$.

## VMC, DMC, AND EXTRAPOLATED CONTACTS

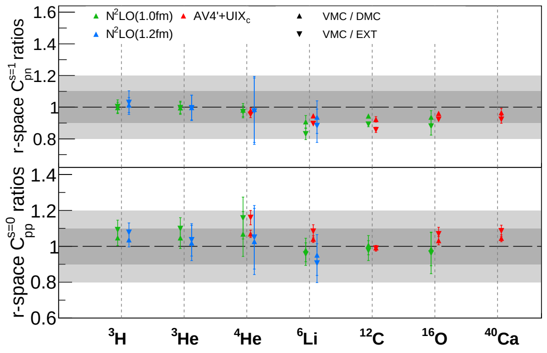


FIG. 3: Ratios of contacts extracted from Variational Monte Carlo (VMC) densities to contacts extracted from Diffusion Monte Carlo (DMC) and extrapolated (EXT = 2×DMC - VMC) distributions.

## CORRELATED FERMI-GAS MODEL

While SRCs are expected to dominate the momentum distributions for momenta above $k_F$, we can see in figure 3 of the main text that scaling in two-body momentum distributions manifests at higher momentum values. To understand this feature and also how the "hardness" of the $NN$ potential affects the onset of this scaling, we built a simple Correlated Fermi-Gas model. We understand delayed scaling to come from the contributions of uncorrelated pairs to the two-body momentum distribution. This model describes a two-component Fermi system with a short-range interaction between different fermions. In this model, 80% of the nucleons are approximated as "free" fermions and the remaining 20% are in a correlated state. The resulting one-body momentum distribution for such a system has two regions: a mean field region with $k < k_F$ and an SRC region with $k > k_F$, as described by Eq. (1),

$$n_{\rm CFG}(k) = \begin{cases} C_1, & 0 < k < k_F, \\ C_2/k^n, & k_F < k < 5\,{\rm fm}^{-1}, \\ 0, & \text{otherwise} \end{cases} \tag{1}$$

where $C_1$ and $C_2$ are normalization constants, and $n$ is usually taken to be $= 4$ [1].

To study the two-body momentum distribution, we perform a Monte-Carlo simulation where we create a "data-base" of nucleons by sampling nucleons in momentum space according to the CFG momentum distribution (Eq. (1)) such that every time a nucleon with momentum $k_1 > k_F$ is sampled, we also sample three center-of-mass momenta values $Q$ (one for each cartesian coordinate) from three gaussian distributions with mean $\mu = 0$ and standard deviation $\sigma = 140\,{\rm MeV/c}$, where this last value was defined by following the results in Ref. [2]. Then, $k_1$ is turned into a vector by sampling a unit vector from a uniform sphere. Accordingly, we create another (correlated) nucleon with momentum:

$$\vec{k}_2 = \vec{Q} - \vec{k}_1 \tag{2}$$

Then, the two-body momentum distributions are created by classifying every resulting NN pair according to one of the following categories:

- the two nucleons are from the Mean-Field: MF-MF
- a nucleon is from the Mean-Field, and the other one is from the high-momentum tail: MF-SRC
- the two nucleons are from the high-momentum tail, but they are not correlated with one another: SRC-SRC (not same pair)
- the two nucleons are from the high-momentum tail, and they belong to an SRC pair: SRC-SRC (same pair)

Figure 4 shows the resulting two-body momentum distribution as a function of $Q$ and relative momentum $q$ ($\vec{q} = (\vec{k_1} - \vec{k_2})/2$) separated into the different types of pairs. For $q < k_F$, the two-body momentum distribution is dominated by MF-MF pairs. As expected, true SRC-SRC pairs (bottom-right plot) dominate the momentum distribution in the high-$q$, low-$Q$ region. As we can see in the top-right plot, as more center-of-mass motion is incorporated into these distributions, we need to go to higher values of $q$ to avoid MF-SRC contributions and access truly short-range correlated nucleons.

In section IV.A of Ref. [3], it was found that SRCs dominate the two-body momentum distribution for $q \gtrsim 1.0 + 0.5 \times Q$. This linear relation is plotted in Figs. 4 and 5 as a diagonal yellow line in the top-right plots and can be understood as the boundary for non-correlated MF-SRC nucleon pairs.

We can study the effect that the "hardness" of the $NN$ potential has on the two-body momentum distribution by changing the value of $n$ in the expression from Eq. (1) (the larger the value of $n$, the softer the interaction is). Figure 5 shows the distributions obtained for $n = 6$ and $n = 8$. For $q$ between $k_F$ and the scaling onset, the two-body momentum distribution is dominated by MF-SRC pairs. As we can see by comparing Figs. 4 and 5, the extent of the MF-SRC pairs is a direct function of the "hardness" of the short-distance $NN$ interaction. If the SRC tail falls faster, MF-SRC pairs will not be able to reach very high-$q$ and the onset will start earlier. Figure 6 shows the ratios MF-SRC/(SRC-SRC)$|_{\text{same pair}}$ and SRC-SRC/(SRC-SRC)$|_{\text{same pair}}$ as a function of $q$ after integrating these 2-body momentum distributions over $Q$, confirming that these ratios fall faster for the "softer" interactions.

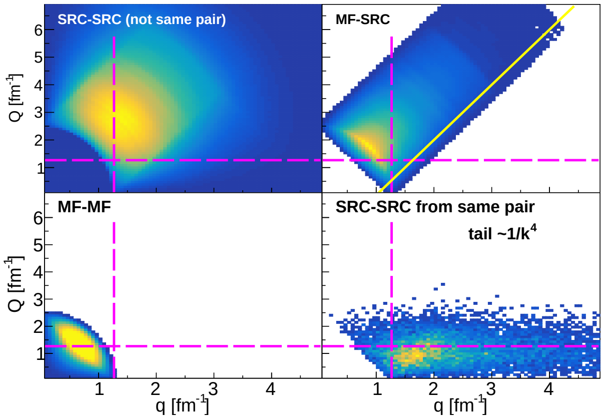


FIG. 4: Two-body momentum distribution as a function of center-of-mass ($Q$) and relative ($q$) momenta corresponding to nucleons that follow Eq. (1) with $n = 4$. The magenta lines correspond to $k_F$. The diagonal yellow line shows, for a given $Q$, the minimum $q$ value above which SRC dominate the two-body momentum distribution [3].

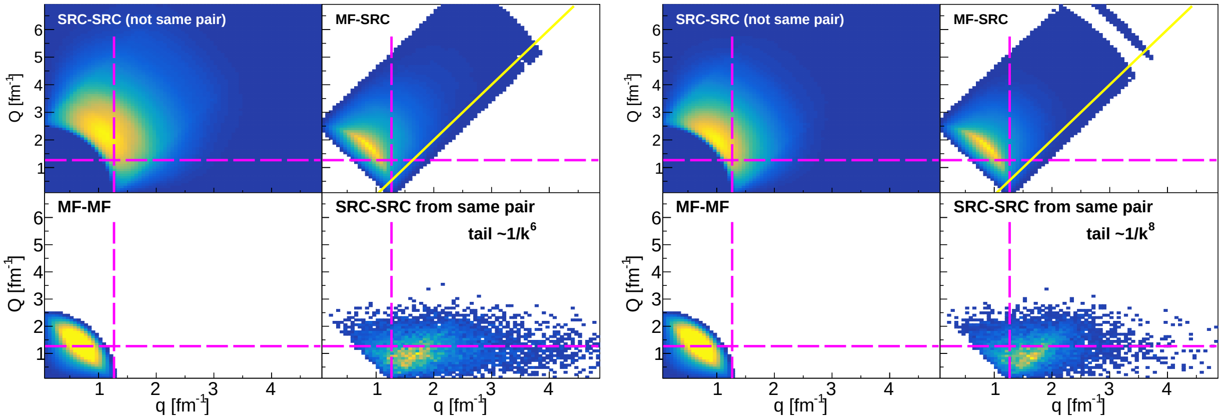


FIG. 5: Same as Fig. 4 but for $n = 6$ (left) and $n = 8$ (right).

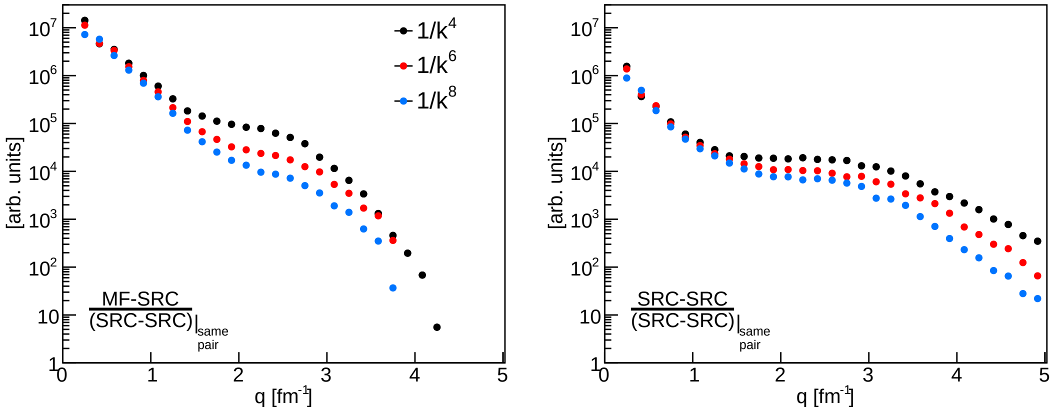


FIG. 6: Ratios MF-SRC/(SRC-SRC)$|_{\text{same pair}}$ and SRC-SRC/(SRC-SRC)$|_{\text{same pair}}$ as a function of $q$ after integrating these 2-body momentum distributions over $Q$.

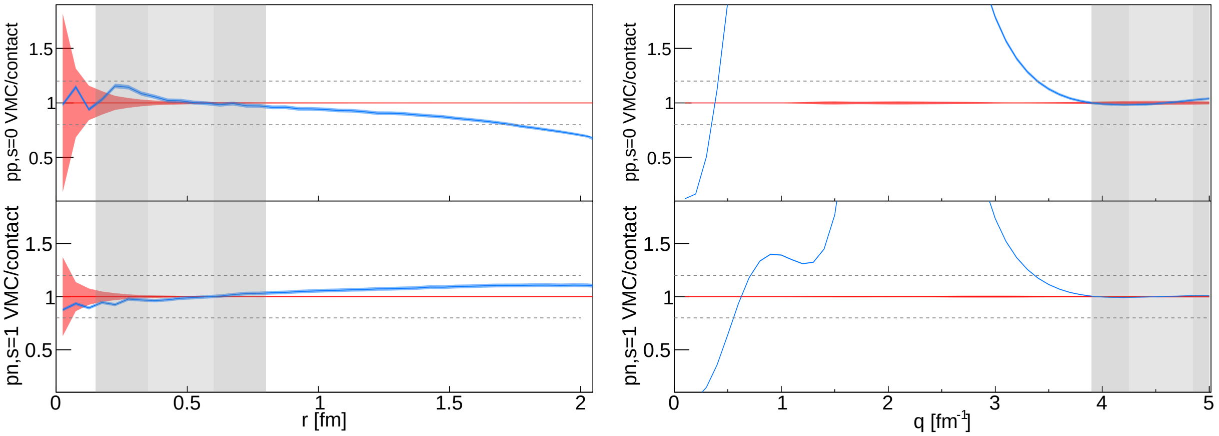


FIG. 7: $^{4}$He fits in coordinate- (left) and momentum-space (right) for the AV4'+UIX$_c$ potential [5, 6]. The fit ranges are shown as vertical gray bands. The darker vertical gray bands represent the ranges within which the fit limits are changed to extract the systematic uncertainty for the contacts. This systematic uncertainty is included in the blue bands The VMC distribution error is added as an uncertainty band to the horizontal red line which has a value of 1. The horizontal dashed lines correspond to a ±20% deviation.

## CONTACT EXTRACTION

Except for the cases of $^{3}$H, $^{3}$He, and $^{12}$C, the nuclear contact terms from AV18+UX used in this analysis were taken from Ref. [4]. Since this analysis was carried out, new AV18+UX $^{3}$H and $^{3}$He VMC distributions were calculated, and the $^{12}$C calculations were updated. These new AV18+UX contacts were extracted following the guidelines described in Ref. [4].

The nuclear contact terms corresponding to the remaining $NN$+3$N$ interactions were extracted by fitting the right- to the left-hand side of Eq. (1) from the main text. That is, we fit the universal two-body wave functions both in coordinate and momentum-space to the corresponding two-body coordinate density or momentum distribution. Since all the spin, isospin projections are not available for the 2-body momentum and coordinate densities, for $C_{pp}^{s=0}$ we fit the total $\rho^{pp}$ assuming that the dominant contribution comes from spin=0 (s-wave) pairs. Furthermore, for $C_{pn}^{s=1}$ ($C_{pn}^{s=0}$) we fit to the T=0 (T=1) pn distributions assuming that the dominant contribution comes from spin=1 (spin=0) pairs with the relevant angular momentum. The figures below illustrate the result of the fits in the case of $^{4}$He. The blue curve corresponds to the ratios:

$$\frac{\rho_A^{NN}(r)}{C_A^{NN,\alpha} \times |\varphi_{NN}^{\alpha}(r)|^2}, \qquad \frac{n_A^{NN}(q)}{C_A^{NN,\alpha} \times |\varphi_{NN}^{\alpha}(q)|^2}, \tag{3}$$

in coordinate and momentum space, respectively. Following the GCF discussion in the main text, these functions scale and are equal to 1 in the regions dominated by short-range correlations. The horizontal red line carries the VMC distribution uncertainty. The fit ranges are shown as vertical gray bands. The uncertainty band in the blue curve corresponds to the systematic uncertainty from the contact extraction, which is determined by repeating the analysis multiple times, varying every fit limit each time within the darker vertical gray bands. The horizontal dashed lines correspond to a ±20% deviation.

[1] O. Hen, L. B. Weinstein, E. Piasetzky, G. A. Miller, M. M. Sargsian, and Y. Sagi, Phys. Rev. C **92**, 045205 (2015).
[2] E. O. Cohen *et al.* (CLAS), Phys. Rev. Lett. **121**, 092501 (2018).
[3] C. Ciofi degli Atti and H. Morita, Phys. Rev. C **96**, 064317 (2017).
[4] R. Weiss, R. Cruz-Torres, N. Barnea, E. Piasetzky, and O. Hen, Phys. Lett. B **780**, 211 (2018).
[5] R. B. Wiringa and S. C. Pieper, Phys. Rev. Lett. **89**, 182501 (2002).
[6] J. E. Lynn, D. Lonardoni, J. Carlson, J.-W. Chen, W. Detmold, S. Gandolfi, and A. Schwenk, (2019), arXiv:1903.12587 [nucl-th] .

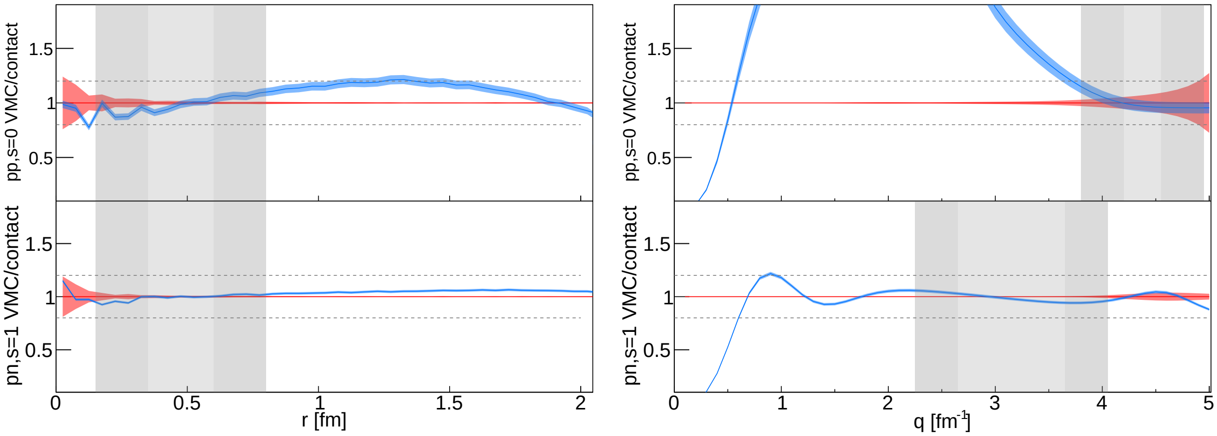


FIG. 8: Same as Fig. 7 but for the $N^2LO$ (1.0 fm, $E1$) potential [7].

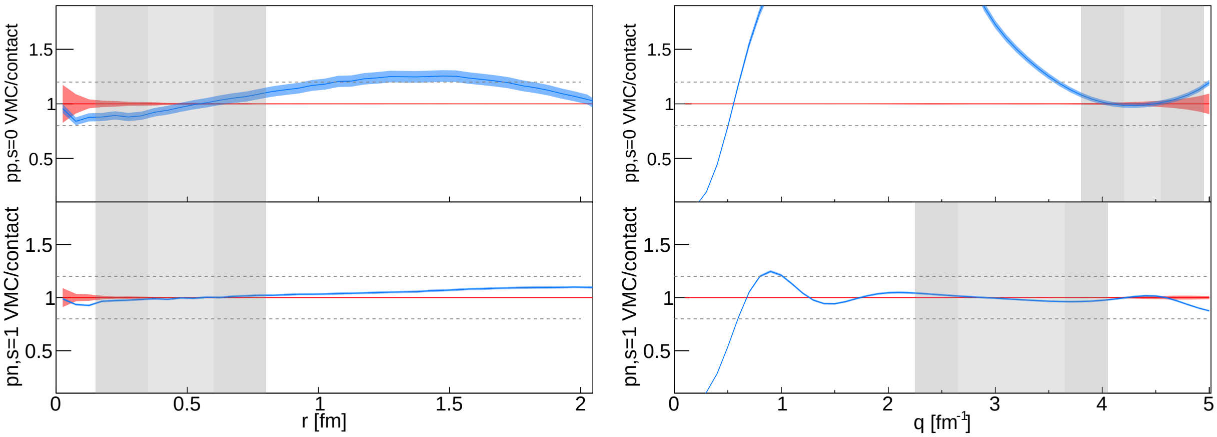


FIG. 9: Same as Fig. 7 but for the $N^2LO$ (1.0 fm, $E\tau$) potential [7].

[7] D. Lonardoni, S. Gandolfi, J. E. Lynn, C. Petrie, J. Carlson, K. E. Schmidt, and A. Schwenk, Phys. Rev. C **97**, 044318 (2018).

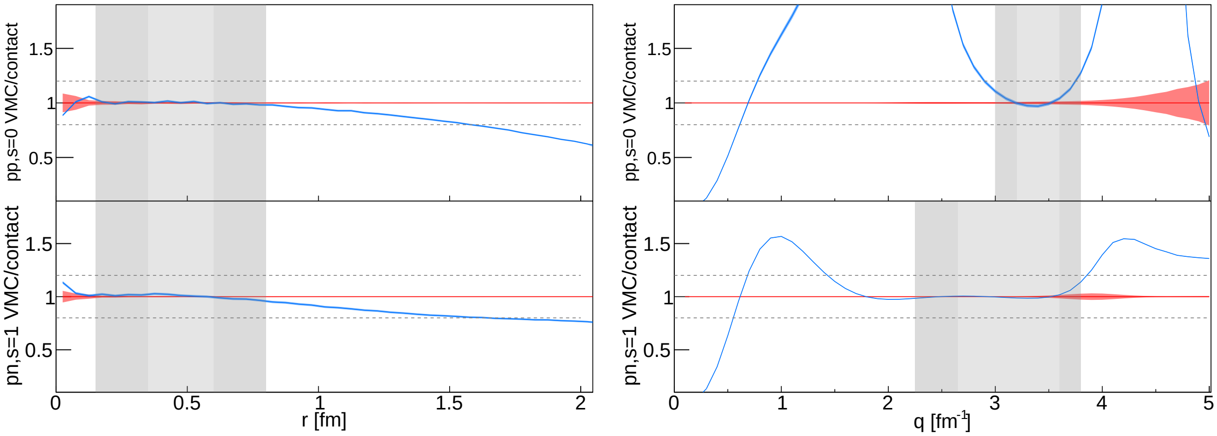


FIG. 10: Same as Fig. 7 but for the N$^2$LO (1.2 fm, $E1$) potential [7].

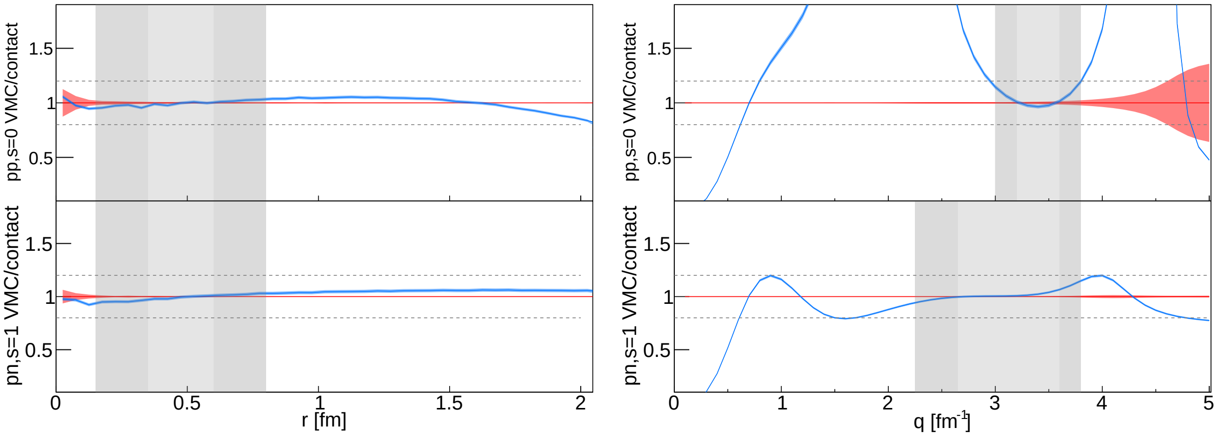


FIG. 11: Same as Fig. 7 but for the N$^2$LO (1.2 fm, $E\tau$) potential [7].
